# Supplementary material for: Open Problems and Modern Solutions for Deep Reinforcement Learning
Source: arXiv:2302.02298 source file (2023-02-05)
Supplement: Supplementary file 1 [file appendix.tex]

\section{Appendix}\label{Appendix}
\subsection{Technical Lemmas for the Proof of Theorem~\ref{corollary_P_star_Ptilder_star}}
\label{appendix_proposition_figure}
\begin{lemma}\label{proposition_figure}
Let $\hat{\mathcal{F}}$, $\mathcal{F}$ and $\bar{\mathcal{F}}$ represent the feasible sets to problem~\eqref{eqn_problem2_mirror}, problem~\eqref{eqn_problem1} and problem~\eqref{eqn_problem_mirrormirror}, respectively. Then, it holds that $\hat{\mathcal{F}} \subseteq \mathcal{F} \subseteq \bar{\mathcal{F}}$.
\end{lemma}
\begin{figure}[htbp]
\centering
\includegraphics[width=5cm]{figures/proposition2.png}
\caption{\small{The illustration for feasible sets of problem~\eqref{eqn_problem2_mirror}--$\hat{\mathcal{F}}$ (light blue), problem~\eqref{eqn_problem1}--$\mathcal{F}$ (red), and problem~\eqref{eqn_problem_mirrormirror}--$\bar{\mathcal{F}}$ (navy blue).}}
\label{fig_three_constraints}
\end{figure}
\begin{proof}
We start by proving the leftmost inclusion. Denote by $\hat{\theta}$ the any feasible solution to problem~\eqref{eqn_problem2_mirror}, i.e., $\hat{\theta} \in \hat{\mathcal{F}}$. By virtue of Proposition~\ref{proposition_U_cP_1-delta} the policy $\pi_{\hat{\theta}}$ is $(1-\delta)$ safe as in Definition~\ref{definition_safety}. In turn, this means that $\hat{\theta}$ is a feasible solution to problem~\eqref{eqn_problem1} as well. Then it holds that $\hat{\theta} \in \mathcal{F}$ for $\forall \hat{\theta} \in \hat{\mathcal{F}}$, thus $\hat{\mathcal{F}} \subseteq \mathcal{F}$.

We now focus on establishing the second inclusion. Denote by $\bar{\theta}$ by any point in $\mathcal{F}$. $\bar{\theta}$ is thus a feasible solution to problem~\eqref{eqn_problem1}, i.e., 
\begin{equation}
\mathbb{P} \left(\bigcap\limits_{t=0}^{T} \{ S_t \in \mathcal{S}_\text{safe}\} \mid \pi_{\bar{\theta}} \right) \geq 1-\delta.
\end{equation}
Observe that the previous inequality is equivalent to
\begin{equation}\label{eqn_lemma1_aux}
\mathbb{P} \left(\sum\limits_{t=0}^{T} \mathbbm{1} \left( S_t \in \mathcal{S}_\text{safe} \right) = T+1 \mid \pi_{\bar{\theta}} \right) \geq 1-\delta.
\end{equation}
Indeed, for the state to belong to $\mathcal{S}_{\text{safe}}$ for all times, all the indicator functions in \eqref{eqn_lemma1_aux} needs to take the value 1.
Since $\sum_{t=0}^T \mathbbm{1} \left( S_t \in \mathcal{S}_\text{safe} \right)$ is a non-negative random variable, it follows that 
\begin{align}\label{eqn_lemma1_aux2}
&\mathbb{E} \left[\sum\limits_{t=0}^{T} \mathbbm{1} \left( S_t \in \mathcal{S}_\text{safe} \right) |\pi_{\bar{\theta}} \right] \\  &\geq \mathbb{P} \left(\sum\limits_{t=0}^{T} \mathbbm{1} \left( S_t \in \mathcal{S}_\text{safe} \right) = T+1 |\pi_{\bar{\theta}} \right) (T+1). \nonumber
\end{align}
Combining \eqref{eqn_lemma1_aux} and \eqref{eqn_lemma1_aux2}, it follows that
\begin{align}
    \mathbb{E} \left[\frac{1}{T+1} \sum\limits_{t=0}^{T} \mathbbm{1} \left( S_t \in \mathcal{S}_\text{safe} \right) |\pi_{\bar{\theta}} \right] \geq 1-\delta.
\end{align}
Hence, $\bar{\theta}$ is a feasible point in $\bar{\mathcal{F}}$ for $\forall \bar{\theta} \in \mathcal{F}$, i.e., $\mathcal{F} \subseteq \bar{\mathcal{F}}$. This completes the proof of Lemma~\ref{proposition_figure}.
\end{proof}

%\subsection{Lemma~\ref{lemma_bound_zero_duality_gap} and its proof}
%\label{appendix_lemma_bound_zero_duality_gap}
%
\begin{lemma}
\label{lemma_bound_zero_duality_gap}
Consider the function $\tilde{P}^\star(\xi)$ defined in \eqref{eqn_problem2}. Let $\xi_0,\xi_1\in\mathbb{R}$. Let $\tilde{\lambda}^\star (\xi_0)$ be the dual optimal solution to \eqref{eqn_problem2} with $\xi=\xi_0$, defined tantamount to \eqref{eqn_dual_solution}.  It holds that
\begin{align}
    \tilde{P}^\star(\xi_1) \leq \tilde{P}^\star(\xi_0) + \tilde{\lambda}^\star (\xi_0) (\xi_0 - \xi_1).
\end{align}
\end{lemma}
\begin{proof}
Recall the definition of the dual problem associated to~\eqref{eqn_problem2}
\begin{align}\label{eqn_min_max}
    \tilde{D}^\star(\xi)= \min\limits_{ \tilde{\lambda}\in\mathbb{R}} \, \max\limits_{\theta\in\mathbb{R}^d} \, V(\theta) +  \tilde{\lambda} (V_c(\theta) - \xi),
\end{align}
where $\tilde{\lambda} \in \Real, \theta \in \Real^d$. It follows from Theorem 3 in \cite{paternain2022safe} that zero duality gap holds for problem \eqref{eqn_problem2}
\begin{align}\label{zero_duality_gap_1}
    \tilde{P}^\star (\xi_1)  = \tilde{D}^\star (\xi_1) = V(\theta^\star (\xi_1)) +  \tilde{\lambda}^\star (\xi_1) (V_c(\theta^\star (\xi_1)) - \xi_1),
\end{align}
where $(\theta^\star (\xi_1), \tilde{\lambda}^\star (\xi_1))$ denote the primal-dual optimal solution of \eqref{eqn_problem2} with $\xi = \xi_1$. Likewise, we can also write 
\begin{align}\label{zero_duality_gap_5}
    \tilde{P}^\star (\xi_0) = V(\theta^\star (\xi_0)) +  \tilde{\lambda}^\star (\xi_0) (V_c(\theta^\star (\xi_0)) - \xi_0),
\end{align}
where the primal-dual solution with respect to $\xi_0$ is denoted by $(\theta^\star (\xi_0), \tilde{\lambda}^\star (\xi_0))$. 
By definition of $\tilde{\lambda}^\star (\xi_1)$, i.e., the minimizer of \eqref{eqn_min_max} with $\xi=\xi_1$, it follows that for any $\lambda>0$ we have that 
\begin{align}
    \tilde{P}^\star(\xi_1)&=V(\theta^\star (\xi_1)) +   \tilde{\lambda}^\star (\xi_1) (V_c(\theta^\star (\xi_1)) - \xi_1) \nonumber \\ 
    &\leq  V(\theta^\star (\xi_1)) +   \lambda (V_c(\theta^\star (\xi_1)) - \xi_1).
\end{align}
In particular, this holds for $\lambda= \tilde{\lambda}^\star(\xi_0)$
\begin{align}
    \tilde{P}^\star(\xi_1) \leq  V(\theta^\star (\xi_1)) +   \tilde{\lambda}^\star(\xi_0) (V_c(\theta^\star (\xi_1)) - \xi_1).
\end{align}

By adding and subtracting $\tilde{\lambda}^\star (\xi_0) \, \xi_0$ to the previous expression yields
\begin{align}\label{zero_duality_gap_2}
   \tilde{P}^\star (\xi_1) &\leq V(\theta^\star (\xi_1)) +  \tilde{\lambda}^\star (\xi_0) (V_c(\theta^\star (\xi_1)) - \xi_0) \nonumber \\
   &+  \tilde{\lambda}^\star (\xi_0) (\xi_0 - \xi_1).
\end{align}

Likewise, $\theta^\star (\xi_0)$ is the primal maximizer of the Lagrangian with $\xi = \xi_0$
\begin{equation}
\theta^\star(\xi_0) = \argmax_{\theta\in\Real^d} V(\theta) + \tilde{\lambda}^\star(\xi_0)\left(V_c(\theta)-\xi_0\right).
\end{equation}
Thus $\tilde{P}^\star(\xi_1)$ in \eqref{zero_duality_gap_2} is upper bounded as
\begin{align}\label{zero_duality_gap_3}
    \tilde{P}^\star(\xi_1) &\leq V(\theta^\star (\xi_0)) +   \tilde{\lambda}^\star (\xi_0) (V_c(\theta^\star (\xi_0)) - \xi_0) \nonumber\\
    &+ \tilde{\lambda}^\star (\xi_0) (\xi_0 - \xi_1).
\end{align}
Substituting \eqref{zero_duality_gap_5} into \eqref{zero_duality_gap_3} reduces to
\begin{align}
    \tilde{P}^\star(\xi_1) \leq \tilde{P}^\star(\xi_0) + \tilde{\lambda}^\star (\xi_0) (\xi_0 - \xi_1).
\end{align}
This completes the proof of Lemma~\ref{lemma_bound_zero_duality_gap}.
\end{proof}

\subsection{Proof of Theorem~\ref{theorem_safe_policy_gradient}}
\label{appendix_theorem_safe_policy_gradient}

We proceed by presenting and proving the following two technical lemmas (Lemma~\ref{lemma_safe_policy_gradient_G1} and Lemma~\ref{lemma_nabla_E_G1_S0_GT_ST-1}).

\begin{lemma}
\label{lemma_safe_policy_gradient_G1}
Given $S_{t-1} \in \mathcal{S}_\text{safe}$ and $G_{t}, t=1,2,\cdots, T-1$ defined in \eqref{def_G_cumulative_product}, it holds that
\begin{align}\label{eqn_recursive_gradient}
\nabla_\theta\mathbb{E}\left[G_{t}\mid S_{t-1}\right] &= \mathbb{E}\left[\nabla_\theta\mathbb{E}\left[G_{t+1}\! \mid \! S_{t}\right]\mathbbm{1}\left(S_{t}\in\mathcal{S}_{\text{safe}}\right) \! \mid \! S_{t-1} \right] \nonumber \\
&+ \mathbb{E}\left[G_{t}\nabla_{\theta}\log\pi_\theta(A_{t-1}\mid S_{t-1}) \mid S_{t-1}\right].
\end{align}
\end{lemma}
\begin{proof}
We start the proof by rewriting the expectation  of $G_1$ with respect to $S_0$ by using the towering property of the expectation
\begin{align}
    \mathbb{E}\left[G_1\mid S_0\right] &=\mathbb{E}\left[\mathbb{E}\left[G_1\mid S_1\right]\mid S_0\right] \nonumber \\
    &= \mathbb{E}\left[\mathbb{E}\left[G_2\mathbbm{1}\left(S_1 \in \mathcal{S}_{\text{safe}}\right)\mid S_1\right]\mid S_0\right], 
\end{align}
where the second equality follows from \eqref{def_G_cumulative_product}. Since $S_1$ is measurable with respect to the $\sigma$-algebra $\mathcal{F}_{1}$ it follows that
\begin{equation}
    \mathbb{E}\left[G_1\mid S_0\right] = \mathbb{E}\left[\mathbb{E}\left[G_2\mid S_1\right] \mathbbm{1}\left(S_1 \in \mathcal{S}_{\text{safe}}\right)\mid S_0\right].
\end{equation}
Rewriting the outer expectation in terms of the probability distribution of $S_1$, the previous expression reduces to
\begin{equation}\label{eqn_conditional_return}
    \mathbb{E}\left[G_1\mid S_0\right] = \int_{\mathcal{S}}\mathbb{E}\left[G_2\mid s_1\right]\mathbbm{1}\left(s_1 \in \mathcal{S}_{\text{safe}}\right) p\left(s_1 \mid S_0\right) \, ds_1.
\end{equation}

Notice that the conditional probability of $s_1$ given $S_0$ can be rewritten as %
\begin{equation}
    p(s_1\mid S_0) = \int_{\mathcal{A}} p(s_1\mid S_0,\,a_0) \pi_{\theta}(a_0\mid S_0) \, da_0.
\end{equation}
Hence, substituting the previous expression into \eqref{eqn_conditional_return} yields
\begin{align}
    \mathbb{E}\left[G_1\mid S_0\right] = \int_{\mathcal{S}\times \mathcal{A}} &\mathbb{E}\left[G_2\mid s_1\right]\mathbbm{1}\left(s_1 \in \mathcal{S}_{\text{safe}}\right) \nonumber  \\
    &p(s_1 \mid S_0, \, a_0) \pi_{\theta}(a_0 \mid S_0) \, ds_1 da_0.
\end{align}
Taking the gradient of the previous expression with respect to the policy parameters $\theta$ results in the following expression
\begin{align}\label{eqn_gradient_1}
    \nabla_\theta \mathbb{E}\left[G_1\mid S_0\right]  &= \int_{\mathcal{S}\times \mathcal{A}}\nabla_{\theta}\left(\mathbb{E}\left[G_2\mid s_1\right]\right)\mathbbm{1}\left(s_1 \in \mathcal{S}_{\text{safe}}\right) \nonumber \\
    & \quad\quad\quad\quad p(s_1 \mid S_0, \, a_0) \pi_{\theta}(a_0\mid S_0) \, ds_1 da_0  \nonumber \\
    &+\int_{\mathcal{S}\times \mathcal{A}}\mathbb{E}\left[G_2\mid s_1\right]\mathbbm{1}\left(s_1 \in \mathcal{S}_{\text{safe}}\right) \nonumber \\
    & \quad\quad\quad\quad p(s_1 \! \mid \! S_0, \, a_0) \nabla_{\theta}\pi_{\theta}(a_0 \! \mid \! S_0) \, ds_1 da_0.
\end{align}
Notice that the first in the right hand side of the previous expression can be presented by
\begin{align}\label{eqn_pre_recursion_1}
&\int_{\mathcal{S}\times \mathcal{A}} \nabla_{\theta}\left(\mathbb{E}\left[G_2\mid s_1\right]\right)\mathbbm{1}\left(s_1 \in \mathcal{S}_{\text{safe}}\right) \nonumber \\
&\quad \quad \quad p(s_1 \mid S_0, \, a_0) \pi_{\theta}(a_0\mid S_0) \, ds_1 da_0  \nonumber \\
&= \mathbb{E}\left[\nabla_\theta\mathbb{E}\left[G_2\mid S_1\right]\mathbbm{1}\left(S_1\in\mathcal{S}_{\text{safe}}\right) \mid S_0 \right].
\end{align}

The second term using the ``log-trick'', i.e. the fact that $\nabla_\theta \pi_{\theta}(a_0\mid S_0) = \pi_{\theta}(a_0\mid S_0) \nabla_\theta \log\pi_\theta(a_0\mid S_0)$ yields
\begin{align}\label{eqn_logtrick}
    &\int_{\mathcal{S}\times \mathcal{A}}\mathbb{E}\left[G_2\mid s_1\right]\mathbbm{1}\left(s_1 \in \mathcal{S}_{\text{safe}}\right) \nonumber \\
    &\quad \quad \quad p(s_1 \mid S_0, \, a_0) \nabla_{\theta}\pi_{\theta}(a_0\mid S_0) \, ds_1 da_0 \nonumber \\
    &=\int_{\mathcal{S}\times \mathcal{A}}\mathbb{E}\left[G_2\mid s_1\right]\mathbbm{1}\left(s_1 \in \mathcal{S}_{\text{safe}}\right) p(s_1 \mid S_0, \, a_0) \nonumber \\
    &\quad \quad \quad \quad \pi_{\theta}(a_0\mid S_0) \nabla_\theta \log\pi_\theta(a_0\mid S_0) \, ds_1 da_0.
\end{align}
Likewise, since $s_1$ is measurable with respect to the $\sigma$-algebra $\mathcal{F}_{1}$, \eqref{eqn_logtrick} can be simplified as follows
\begin{align}
    &\int_{\mathcal{S}\times \mathcal{A}}\mathbb{E}\left[G_2\mid s_1\right]\mathbbm{1}\left(s_1 \in \mathcal{S}_{\text{safe}}\right) p(s_1 \mid S_0, \, a_0) \nonumber \\
    &\quad \quad \quad \pi_{\theta}(a_0\mid S_0) \nabla_\theta \log\pi_\theta(a_0\mid S_0) \, ds_1 da_0 \nonumber \\
    &=\int_{\mathcal{S}\times \mathcal{A}}\mathbb{E}\left[G_2\mathbbm{1}\left(s_1 \in \mathcal{S}_{\text{safe}}\right)\mid s_1\right] p(s_1 \mid S_0, \, a_0) \nonumber \\
    &\quad \quad \quad \quad \pi_{\theta}(a_0\mid S_0) \nabla_\theta \log\pi_\theta(a_0\mid S_0) \, ds_1 da_0 \nonumber \\
    &=\int_{\mathcal{S}\times \mathcal{A}}\mathbb{E}\left[G_1 \mid s_1\right] p(s_1 \mid S_0, \, a_0) \pi_{\theta}(a_0\mid S_0) \nonumber \\
    &\quad \quad \quad \quad \nabla_\theta \log\pi_\theta(a_0\mid S_0) \, ds_1 da_0.
\end{align}
Notice that the previous expression is equivalent to
\begin{align}
    &\int_{\mathcal{S}\times \mathcal{A}}\mathbb{E}\left[G_1 \mid s_1\right] p(s_1 \mid S_0, \, a_0) \pi_{\theta}(a_0\mid S_0) \nonumber \\
    &\quad \quad \quad \nabla_\theta \log\pi_\theta(a_0\mid S_0) \, ds_1 da_0 \nonumber  \\
    &= \mathbb{E}\left[\mathbb{E}\left[G_1 \mid S_1\right] \nabla_\theta \log\pi_\theta(A_0\mid S_0) \mid S_0 \right].
\end{align}
Since $\log\pi_\theta(A_0\mid S_0)$ is measurable given $S_1$, the expression above can be rewritten as
\begin{align}
    &\mathbb{E}\left[\mathbb{E}\left[G_1 \mid S_1\right] \nabla_\theta \log\pi_\theta(A_0\mid S_0) \mid S_0 \right] \nonumber \\
    &= \mathbb{E}\left[\mathbb{E}\left[G_1 \nabla_\theta \log\pi_\theta(A_0\mid S_0) \mid S_1\right]  \mid S_0 \right].
\end{align}
Using the towering property of the expectation the previous expressions yield
\begin{align}\label{eqn_pre_recursion_2}
   &\int_{\mathcal{S}\times \mathcal{A}}\mathbb{E}\left[G_2\mid s_1\right]\mathbbm{1}\left(s_1 \in \mathcal{S}_{\text{safe}}\right) p(s_1 \mid S_0, \, a_0) \nonumber \\
   &\quad \quad \quad \nabla_{\theta}\pi_{\theta}(a_0\mid S_0) \, ds_1 da_0 \nonumber \\
   &= \mathbb{E}\left[G_1 \nabla_\theta \log\pi_\theta(A_0\mid S_0) \mid S_0 \right]. 
\end{align}
Then, combining \eqref{eqn_pre_recursion_1} with \eqref{eqn_pre_recursion_2} yields
\begin{align}\label{eqn_appendix_nabla_E_G1_S0}
\nabla_\theta\mathbb{E}\left[G_1\mid S_0\right] &= \mathbb{E}\left[\nabla_\theta\mathbb{E}\left[G_2\mid S_1\right]\mathbbm{1}\left(S_1\in\mathcal{S}_{\text{safe}}\right) \mid S_0 \right] \nonumber \\
&+ \mathbb{E}\left[G_1\nabla_{\theta}\log\pi_\theta(A_0\mid S_0)\mid S_0\right].
\end{align}
Repeating the process above $i$ times for $1 \leq i \leq T-1$, we obtain the following recursive definition of the gradient of the probability in \eqref{eqn_problem1} with respect to $\theta$
\begin{align}
\nabla_\theta\mathbb{E}\left[G_{i}\mid S_{i-1}\right] &= \mathbb{E}\left[\nabla_\theta\mathbb{E}\left[G_{i+1}\! \mid \! S_{i}\right]\mathbbm{1}\left(S_{i}\in\mathcal{S}_{\text{safe}}\right) \! \mid \! S_{i-1} \right]  \nonumber \\
&+ \mathbb{E}\left[G_{i}\nabla_{\theta}\log\pi_\theta(A_{i-1}\mid S_{i-1})\mid S_{i-1}\right].
\end{align}
This completes the proof of Lemma~\ref{lemma_safe_policy_gradient_G1}.
\end{proof}
%
%
%
%
%
%
%
%
%
% \santiago{Now that you are just presenting the Lemmas you don't really need this connecting sentence.}
% %
% {\color{red}{
% Note that the recursive relationship between the gradients of consecutive $G_t$ allows to unwrap the gradient of $\mathbb{E}\left[G_1\mid S_0\right]$ in terms of $G_2,\ldots,G_T$. In particular, in each step of the recursion a new term of the form $ \mathbb{E}\left[G_{t}\nabla_{\theta}\log\pi_\theta(A_{t-1}\mid S_{t-1})\mid S_{t-1}\right]$ is introduced. We state in the following lemma the final expression of the unwrapping.}}
%
\begin{lemma}
\label{lemma_nabla_E_G1_S0_GT_ST-1}
Given $S_{t-1} \in \mathcal{S}_\text{safe}$ and $G_{t}, t=1,2,\cdots, T-1$ defined in \eqref{def_G_cumulative_product}, it holds that
\begin{align}\label{eqn__nabla_E_G1_S0_GT_ST-1}
    \nabla_\theta\mathbb{E}\left[G_1\mid S_0\right] &=\sum\limits_{t=0}^{T-2}\mathbb{E}\left[G_1\nabla_{\theta}\log\pi_\theta(A_t\mid S_t)\mid S_0\right] \nonumber \\ &+\mathbb{E}\left[\nabla_\theta\mathbb{E}\left[G_T \! \mid \! S_{T-1}\right]\! \prod_{t=1}^{T-1} \! \mathbbm{1}\left(\! S_{t}\in\mathcal{S}_{\text{safe}} \!\right) \! \mid \! S_0\right]. 
\end{align}
\end{lemma}
\begin{proof}
We proceed by employing Lemma~\ref{lemma_safe_policy_gradient_G1} to derive the gradient of the expectation of $G_1$ and $G_2$, respectively 
\begin{align}\label{eqn_mainbody_nabla_E_G1_S0}
\nabla_\theta\mathbb{E}\left[G_{1}\mid S_{0}\right] &= \mathbb{E}\left[\nabla_\theta\mathbb{E}\left[G_{2}\mid S_{1}\right]\mathbbm{1}\left(S_{1}\in\mathcal{S}_{\text{safe}}\right) \mid S_{0} \right] \nonumber \\ 
&+ \mathbb{E}\left[G_{1}\nabla_{\theta}\log\pi_\theta(A_{0}\mid S_{0})\mid S_{0}\right].
\end{align}
\begin{align}\label{eqn_mainbody_nabla_E_G2_S1}
   \nabla_\theta\mathbb{E}\left[G_2\mid S_1\right] &= \mathbb{E}\left[\nabla_\theta\mathbb{E}\left[G_3\mid S_2\right]\mathbbm{1}\left(S_2\in\mathcal{S}_{\text{safe}}\right) \mid S_1 \right] \nonumber \\
   &+ \mathbb{E}\left[G_2\nabla_{\theta}\log\pi_\theta(A_1\mid S_1)\mid S_1\right]. 
\end{align}
Then, substituting \eqref{eqn_mainbody_nabla_E_G2_S1} into \eqref{eqn_mainbody_nabla_E_G1_S0} yields
\begin{align}\label{eqn_mainbody_nabla_E_G1_S0_2}
    &\nabla_\theta\mathbb{E} [G_1\mid S_0 ] \nonumber \\
    &=\mathbb{E}[\mathbb{E} [\nabla_\theta\mathbb{E} [G_3\mid S_2 ]  \mathbbm{1} (S_2\in\mathcal{S}_{\text{safe}} ) \mid S_1  ]\mathbbm{1} (S_1\in\mathcal{S}_{\text{safe}} ) \nonumber \\
    &+\mathbb{E} [G_2\nabla_{\theta}\log\pi_\theta(A_1\mid S_1)\mid S_1 ]  \mathbbm{1} (S_1\in\mathcal{S}_{\text{safe}} ) \mid S_0] \nonumber \\
    &+\mathbb{E} [G_1\nabla_{\theta}\log\pi_\theta(A_0\mid S_0)\mid S_0 ].
\end{align}
As $\mathbbm{1}\left(S_1\in\mathcal{S}_{\text{safe}}\right)$ is measurable given $S_1$, the previous equation can be transformed to
\begin{align}
    &\nabla_\theta\mathbb{E}\left[G_1\mid S_0\right] \nonumber \\
    &= \mathbb{E}[\mathbb{E}\left[\nabla_\theta\mathbb{E}\left[G_3\mid S_2\right]\mathbbm{1}\left(S_2\in\mathcal{S}_{\text{safe}}\right) \mathbbm{1}\left(S_1\in\mathcal{S}_{\text{safe}}\right) \mid S_1 \right] \nonumber \\
    & +\mathbb{E}\left[G_2\nabla_{\theta}\log\pi_\theta(A_1\mid S_1) \mathbbm{1}\left(S_1\in\mathcal{S}_{\text{safe}}\right) \mid S_1\right] \mid S_0] \nonumber \\ 
    & + \mathbb{E}\left[G_1\nabla_{\theta}\log\pi_\theta(A_0\mid S_0)\mid S_0\right].
\end{align}
By definition of $G_1$ we can simplify the second term of the right hand side of the previous equation. Then we have
\begin{align}\label{eqn_appendix__nabla_E_G1_S0_3}
    &\nabla_\theta\mathbb{E}\left[G_1\mid S_0\right] \nonumber \\
    &= \mathbb{E}[\mathbb{E}\left[\nabla_\theta\mathbb{E}\left[G_3\mid S_2\right]\mathbbm{1}\left(S_2\in\mathcal{S}_{\text{safe}}\right) \mathbbm{1}\left(S_1\in\mathcal{S}_{\text{safe}}\right) \mid S_1 \right] \nonumber \\
    &+\mathbb{E}\left[G_1\nabla_{\theta}\log\pi_\theta(A_1\mid S_1) \mid S_1\right] \mid S_0] \nonumber \\
    &+ \mathbb{E}\left[G_1\nabla_{\theta}\log\pi_\theta(A_0\mid S_0)\mid S_0\right].
\end{align}
Using the towering property of the expectation \eqref{eqn_appendix__nabla_E_G1_S0_3} reduces to
\begin{align}
    &\nabla_\theta\mathbb{E}\left[G_1\mid S_0\right] \nonumber \\
    &= \mathbb{E}\left[\nabla_\theta\mathbb{E}\left[G_3\mid S_2\right]\mathbbm{1}\left(S_2\in\mathcal{S}_{\text{safe}}\right) \mathbbm{1}\left(S_1\in\mathcal{S}_{\text{safe}}\right) \mid S_0\right] \nonumber \\
    & +\mathbb{E}\left[G_1\nabla_{\theta}\log\pi_\theta(A_1\mid S_1) \mid S_0\right] \nonumber \\
    &+ \mathbb{E}\left[G_1\nabla_{\theta}\log\pi_\theta(A_0\mid S_0)\mid S_0\right].
\end{align}
Then repeatedly unwrapping $\nabla_\theta\mathbb{E}\left[G_1\mid S_0\right]$ in terms of $G_3,\ldots,G_T$ by Lemma~\ref{lemma_safe_policy_gradient_G1} yields
\begin{align}
    &\nabla_\theta\mathbb{E}\left[G_1\mid S_0\right] \nonumber \\ &=\mathbb{E} [\nabla_\theta\mathbb{E}\left[G_T\mid S_{T-1}\right] \mathbbm{1}\left(S_{T-1}\in\mathcal{S}_{\text{safe}}\right) \nonumber \\
    &\quad\cdots \mathbbm{1}\left(S_2\in\mathcal{S}_{\text{safe}}\right) \mathbbm{1}\left(S_1\in\mathcal{S}_{\text{safe}}\right) \mid S_0] \nonumber \\
    & +\mathbb{E}\left[G_1\nabla_{\theta}\log\pi_\theta(A_{T-2}\mid S_{T-2}) \mid S_0\right]+ \cdots \nonumber \\
    &+ \mathbb{E}\left[G_1\nabla_{\theta}\log\pi_\theta(A_0\mid S_0)\mid S_0\right] \nonumber \\
    &=\sum\limits_{t=0}^{T-2}\mathbb{E}\left[G_1\nabla_{\theta}\log\pi_\theta(A_t\mid S_t)\mid S_0\right] \nonumber \\
    &+ \mathbb{E}\left[\nabla_\theta\mathbb{E}\left[G_T\mid S_{T-1}\right]\prod_{t=1}^{T-1}\mathbbm{1}\left(S_{t}\in\mathcal{S}_{\text{safe}}\right) \mid S_0\right].
\end{align}
This completes the proof of Lemma~\ref{lemma_nabla_E_G1_S0_GT_ST-1}.
\end{proof}

We are now in conditions to prove Theorem~\ref{theorem_safe_policy_gradient}. We start by rewriting the probability of remaining safe in terms of $G_0$ defined in  \eqref{def_G_cumulative_product}. By definition of probability we have
\begin{align}
    &\mathbb{P} \left(\bigcap\limits_{t=0}^{T} \{ S_t \in \mathcal{S}_\text{safe}\} |\pi_\theta, S_0 \right) \nonumber \\
    &= \mathbb{E} \left[\mathbbm{1} \left(\bigcap\limits_{t=0}^{T} \{ S_t \in \mathcal{S}_\text{safe}  \}\right) |\pi_\theta, S_0 \right].
\end{align}
Note that the indicator function in the previous expression takes the value one, if and only if each $S_t\in\mathcal{S}_{\text{safe}}$. Hence, it is possible to rewrite the previous expression in terms of the product of indicator functions of states satisfying the safety condition at each time
\begin{align}\label{eqn_safe_policy_gradient_G0}
    \mathbb{P} \left(\bigcap\limits_{t=0}^{T} \{ S_t \in \mathcal{S}_\text{safe}\} |\pi_\theta, S_0 \right) &= \mathbb{E} \left[\! \prod\limits_{t=0}^{T} \! \mathbbm{1} (S_t \in \mathcal{S}_\text{safe}) |\pi_\theta, S_0 \right] \nonumber \\
    &= \mathbb{E}\left[G_0 | S_0\right],
\end{align}
where $\pi_\theta$ is omitted in the last equation for simplicity. By virtue of $S_0 \in \mathcal{S}_\text{safe}$, we obtain $ \mathbb{E}[G_0 | S_0] = \mathbb{E}[G_1 \cdot \mathbbm{1} (S_0 \in \mathcal{S}_\text{safe}) | S_0]=\mathbb{E}[G_1 | S_0].$ Then, using \eqref{eqn_safe_policy_gradient_G0}, the gradient of the probability of remaining safe reduces to
\begin{equation}\label{eqn_safe_policy_gradient_G1}
    \nabla_\theta \mathbb{P} \left(\bigcap\limits_{t=0}^{T} \{ S_t \in \mathcal{S}_\text{safe}\} |\pi_\theta, S_0 \right)=\nabla_\theta \mathbb{E}\left[G_1 | S_0\right].
\end{equation}
In Lemma~\ref{lemma_safe_policy_gradient_G1} we derive a recursive relationship for the gradient of $\mathbb{E}\left[G_t\mid S_{t-1}\right], t=1,2,\cdots, T-1 $. By virtue of Lemma~\ref{lemma_nabla_E_G1_S0_GT_ST-1}, to complete the proof of the result it suffices to establish that 
\begin{align}\label{eqn_thing_to_show}
    &\mathbb{E}\left[\nabla_\theta\mathbb{E}\left[G_T\mid S_{T-1}\right]\prod_{t=1}^{T-1}\mathbbm{1}\left(S_{t}\in\mathcal{S}_{\text{safe}}\right) \mid S_0\right] \nonumber \\
    &= \mathbb{E}\left[G_1\nabla_\theta \log \pi_{\theta}(A_{T-1} \mid S_{T-1})\mid S_0\right]. 
\end{align}
We establish this result next. Let us start by working with the gradient of the inner expectation on the left hand side of the previous expression. 

Using the fact that $G_T = \mathbbm{1}\left(S_T\in\mathcal{S}_{\text{safe}}\right)$ and the definition of expectation one can write $\nabla_\theta\mathbb{E}\left[G_T\mid S_{T-1}\right]$ in the left hand side of the previous expression as
\begin{equation}\label{eqn_nabla_G_T}
   \nabla_\theta\mathbb{E}\left[G_T\mid S_{T-1}\right] = \nabla_\theta \int_{\mathcal{S}} \mathbbm{1} (s_T \in \mathcal{S}_\text{safe}) p(s_T | S_{T-1}) \, ds_T, 
\end{equation}
where $p\left(s_T\mid S_{T-1}\right)$ denotes the conditional probability of $S_T$ given $S_{T-1}$. Marginalizing the probability distribution it follows that 
\begin{align}
    p(s_T | S_{T-1}) \! = \! \int_{\mathcal{A}} \! p(s_T | S_{T-1}, a_{T-1})  \pi_{\theta}(a_{T-1} | S_{T-1}) da_{T-1}.
\end{align}
Consequently, \eqref{eqn_nabla_G_T} can be converted to
\begin{align}
   &\nabla_\theta\mathbb{E}\left[G_T\mid S_{T-1}\right] \nonumber \\
   &= \nabla_\theta\int_{\mathcal{S}\times \mathcal{A}} \mathbbm{1}\left(s_T \in \mathcal{S}_{\text{safe}}\right) p(s_T \mid S_{T-1}, \, a_{T-1}) \nonumber \\
   &\quad \quad \quad \quad \quad \quad \pi_{\theta}(a_{T-1}\mid S_{T-1}) \, ds_T da_{T-1}.
\end{align}
Note that in the previous expression, the only term dependent on $\theta$ is the policy, hence we have that
\begin{align}
   \nabla_\theta\mathbb{E}\left[G_T\mid S_{T-1}\right]  =\int_{\mathcal{S}\times \mathcal{A}}\! &\mathbbm{1}\left(s_T \in \mathcal{S}_{\text{safe}}\right) p(s_T \! \mid \! S_{T-1}, \, a_{T-1}) \nonumber \\
   &\nabla_\theta\pi_{\theta}(a_{T-1}\mid S_{T-1}) \, ds_T da_{T-1}. 
\end{align}
Applying the ``log-trick'' to the right hand side of the previous equation yields
\begin{align}
   &\nabla_\theta\mathbb{E}\left[G_T\mid S_{T-1}\right] \nonumber \\ &=\int_{\mathcal{S}\times \mathcal{A}}\mathbbm{1}\left(s_T \in \mathcal{S}_{\text{safe}}\right) p(s_T \mid S_{T-1}, \, a_{T-1}) \nonumber \\
   &\quad~\pi_{\theta}(a_{T-1}\mid S_{T-1}) \nabla_\theta\log\pi_{\theta}(a_{T-1}\mid S_{T-1}) \, ds_T da_{T-1}. 
   \end{align}
Since $p\left(s_T\mid S_{T-1},a_{T-1}\right)\pi_\theta\left(a_{T-1}\mid S_{T-1}\right) = p\left(s_T,a_{T-1}\mid S_{T-1}\right)$ is the joint probability distribution of $S_{T}$ and $A_{T-1}$ given $S_{T-1}$ the previous expression can be rewritten as 
\begin{equation}
    \nabla_\theta\mathbb{E}\left[G_T\mid S_0\right]  =\mathbb{E}\left[G_T\nabla_{\theta}\log\pi_\theta(A_{T-1}\mid S_{T-1})\mid S_{T-1}\right]. 
\end{equation}

Since $S_1,\ldots, S_{T-1}$ are measurable with respect to $S_{T-1}$ it follows that 
\begin{align}
   &\nabla_\theta\mathbb{E}\left[G_T\mid S_0\right] \prod_{t=1}^{T-1}\mathbbm{1}\left(S_{t}\in\mathcal{S}_{\text{safe}}\right) \nonumber \\
   &=\mathbb{E}\left[G_1\nabla_{\theta}\log\pi_\theta(A_{T-1}\mid S_{T-1})\mid S_{T-1}\right],
\end{align}
where we have used that $G_1 = G_T\prod_{t=1}^{T-1}\mathbbm{1}\left(S_{t}\in\mathcal{S}_{\text{safe}}\right)$. Substituting the previous expression in the left hand side of \eqref{eqn_thing_to_show} it follows that 
\begin{align}
    &\mathbb{E}\left[\nabla_\theta\mathbb{E}\left[G_T\mid S_{T-1}\right]\prod_{t=1}^{T-1}\mathbbm{1}\left(S_{t}\in\mathcal{S}_{\text{safe}}\right) \mid S_0\right] \nonumber \\
    &=\mathbb{E}\left[\mathbb{E}\left[G_1\nabla_\theta \log \pi_{\theta}(A_{T-1} \mid S_{T-1}) \mid S_{T-1}\right]\mid S_0\right]. 
\end{align}
The law of total expectation completes the result claimed in \eqref{eqn_thing_to_show} and therefore completes the proof of Theorem~\ref{theorem_safe_policy_gradient}.
